# Supplementary material for: QuReed
Source: arXiv:2406.07638 source file (2024-06-11)
Supplement: Supplementary file 1 [file 01_beamsplitter.tex]

\subsection{Ideal Non-Polarizing Beam-Splitter}

Beam-Splitter is a rudimentary device in the optical laboratory. Here we describe the action of the ideal beam splitter as well as the implementation in \gls{sim} framework.

Suppose we have two single-photon states $\ket{\psi_a}$ and $\ket{\psi_b}$ with Gaussian temporal profiles. The temporal modes can be described by wave packets, and the temporal overlap will affect the interaction at the beam splitter.

Let the temporal profiles of the wave packets be given by a Gaussian functions:
\begin{align}
    \psi_a(t) &= \frac{1}{\sqrt{\sigma_a\sqrt{\pi}}}e^{\frac{(t-t_a)^2}{2\sigma_a^2}} e^{i\omega_a t},&
    \psi_b(t) &= \frac{1}{\sqrt{\sigma_b\sqrt{\pi}}}e^{\frac{(t-t_b)^2}{2\sigma_b^2} e^{i\omega_b t}}.
\end{align}

The values $\omega_a$ and $\omega_b$ represent the central frequencies of these two packets and times $t_a$ and $t_b$ represent central times respectively.

Now we consider standard operator for the beam splitter (as seen in \cite{makarov2022theory}, equation 17):

\begin{equation}
    \hat U_{BS} = \exp(i\phi(\hat a^\dagger_1 \hat a_2 - \hat a_1 \hat a^\dagger_2)),
\end{equation}

where we consider the action of 50:50 beam splitter, thus setting the $\phi=\pi/4$.

Now we consider possible cases for the input states. If only one photon enters beam splitter at port A, then the output can simply be computed as:

\begin{align}
    \begin{split}
        \ket{\psi_{out}} = \hat U_{BS} \ket{1}_{A, t_0}\ket{0}_{A, t_0} = ()
    \end{split}
\end{align}

The overlap integral between the two temporal modes is:
\begin{equation}
    \Lambda = \int_{-\infty}^{\infty}\psi_a^*(t)\psi_b(t)dt,
\end{equation}
which for given Gaussian profiles, can be computed as:
\begin{equation}
    \Lambda = \exp(-\frac{(t_a-t_b)^2}{4\sigma_a\sigma_b})\cdot \exp(-\frac{\sigma_a^2\sigma_b^2\Delta\omega^2}{\sigma_a^2 + \sigma_b^2})
\end{equation}

Now consider a beam split operator (as seen in \cite{makarov2022theory} equation 17):
\begin{align}
\hat U_{BS} &= \hat D^\dagger&
\hat D &= e^{\eta \hat L_+ - \eta^* \hat L_-},
\end{align}

with the $\hat L_-=\hat a^\dagger_1 \hat a_2$ and $\hat L_+ = \hat a_2^\dagger \hat a_1$.

Lets consider a case where the two incoming photons $\ket{1}_{a,t_1}$ and $\ket{1}_{b,t_2}$ are totally distinguishable ($\Lambda = 0 $). In practice when each of these photons interacts with the beam-splitter, the beam-splitter would assume vacuum state in the other port, which would result in the following outputs:
\begin{align}\label{eq:non_overlapping_bs}
    &\hat U_{BS} (\ket{1}_{a,t_1}\ket{0}_{b,t_1}), &
    &\hat U_{BS} (\ket{0}_{a,t_2}\ket{1}_{b,t_2}).
\end{align}

If both packets arrive at the same time, then the operation is trivial $\hat U_{BS} \ket{1}_{a,t_0}\ket{1}_{b,t_0}$. In these two cases, the central Gaussian times are not affected. It is interesting to study, what happens to packets which arrive with some delay $\tau=t_2-t_1$ such that the temporal profiles of the two packets partially overlaps ($0<\Lambda < 1$). In our model we assume that based on the overlap factor $\Lambda$, beam splitter acts on the overlapping spaces and partially on the spaces separately. In this case we need to introduce two new vacuum Fock spaces like in equation \eqref{eq:non_overlapping_bs}. In effect we need to compute an operator which acts on four Fock spaces:

\begin{equation}
    \hat U'_{BS} = \Lambda \hat U_{BS, i} +(1-\Lambda) \hat U_{BS, d},
\end{equation}

where first term represents the proportional overlapping (distinguishable) term and the second proportional non-overlapping (indistinguishable) term. Each of the two terms need to operate on four Fock spaces.

\begin{align}
    \hat U_{BS, d} &= \exp(i\phi (a_1^\dagger a_2 + a_1 a_2^\dagger)) \otimes \hat I_3 \otimes \hat I_4, \\
    \hat U_{BS, i} &= \exp(i\phi (a_1^\dagger a_3 + a_1 a_3^\dagger)) \otimes
    \exp(i\phi (a_2^\dagger a_4 + a_2 a_4^\dagger)),
\end{align}
where we consider the following auxiliary spaces $\ket{0}_3$ and $\ket{0}_4$ in a vacuum state. For a ideal 50:50 beam splitter we set $\phi=\frac{\pi}{4}$.Now we have two operators which we apply in the case of either non-overlapping photons($\hat U_{BS}$, with vacuum state), fully overlapping photons ($\hat U_{BS}$, with respective Fock state) and partially overlapping photons($\hat U'_{BS}$, with two vacuum states).

\begin{minted}{Python}
class NonPolarizingBeamSplitter(GenericDevice):
    ## ... Ports ...
    def des():
        pass
\end{minted}
